# Supplementary material for: InfinityGAN: Towards Infinite-Pixel Image Synthesis
Source: arXiv:2104.03963 source file (2022-03-11)
Supplement: Supplementary file 1 [file supp-fig_alis_artifacts.tex]

\begin{figure}[H]
    \vspace{-2em}
    \centering
    \setlength{\tabcolsep}{0pt}
    \begin{tabular}{c c c c}
        \includegraphics[width=0.22\linewidth]{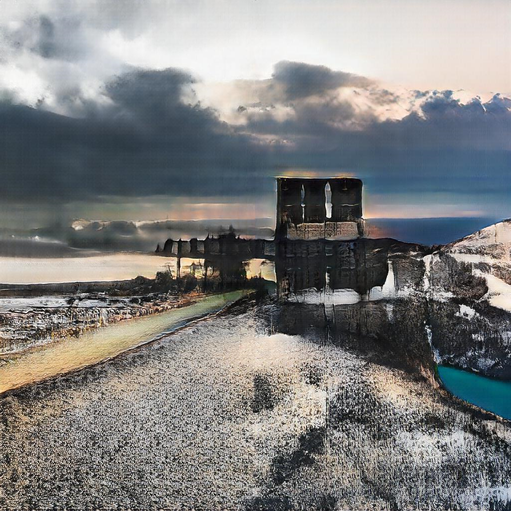} \hfill & \hfill
        \includegraphics[width=0.22\linewidth]{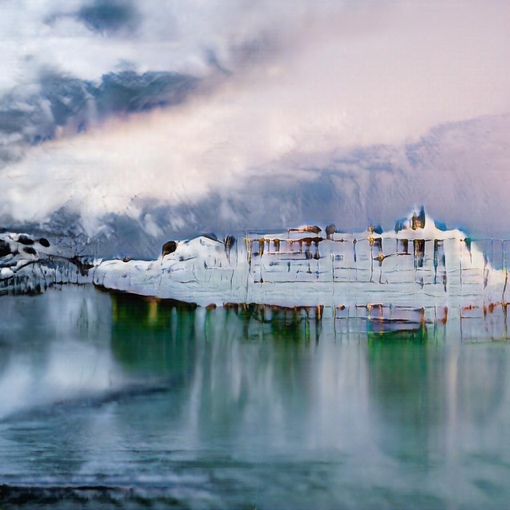} \hfill & \hfill
        \includegraphics[width=0.22\linewidth]{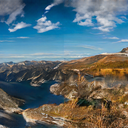} \hfill & \hfill
        \includegraphics[width=0.22\linewidth]{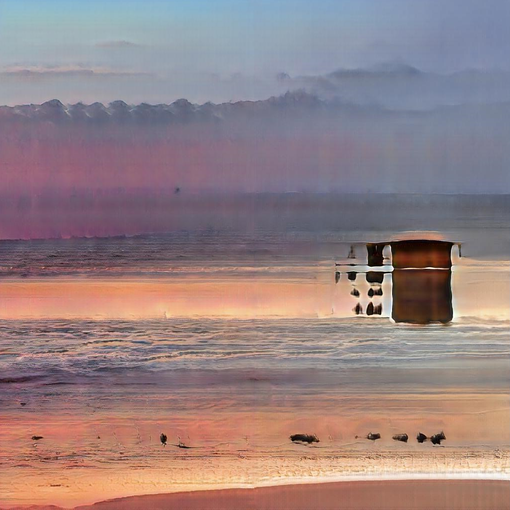}
        \\
        \includegraphics[width=0.22\linewidth]{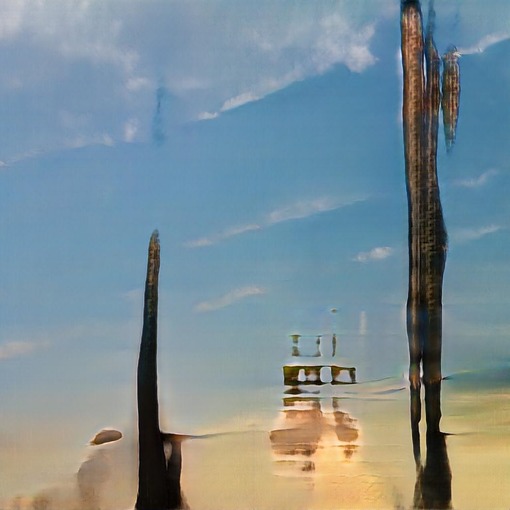} \hfill & \hfill
        \includegraphics[width=0.22\linewidth]{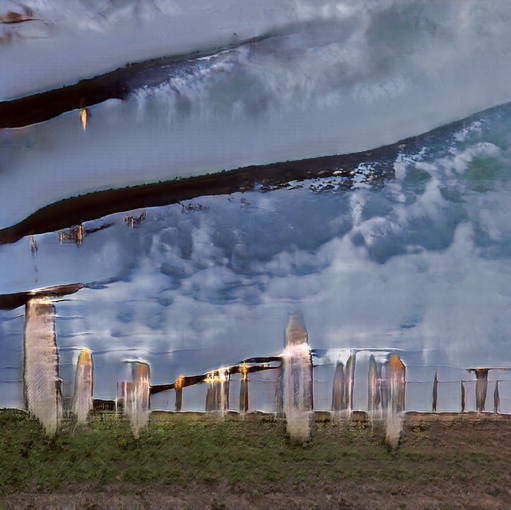} \hfill & \hfill
        \includegraphics[width=0.22\linewidth]{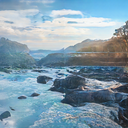} \hfill & \hfill
        \includegraphics[width=0.22\linewidth]{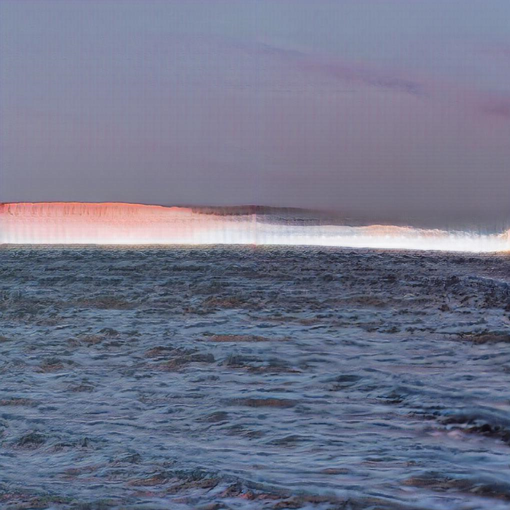}
        \\
        \cmidrule(lr){1-2}
        \cmidrule(lr){3-3}
        \cmidrule(lr){4-4}
        \multicolumn{2}{c}{Blocky Artifacts} & Discontinuity & Lattice
        Artifacts
    \end{tabular}
    
    \vspace{-1em}
    
    \caption{
    \textbf{ALIS can suffer from blocky artifacts, inter-patch discontinuity and lattice artifacts.} 
    We train ALIS with the official implementation at 1024$\times$1024 resolution. 
    We focus on the failure cases caused by COCO-GAN-based generation-by-parts framework, which artificially enforces the learned inter-patch continuity with adversarial learning.
    % Note that these samples are focusing on the failure cases, which do not represent the overall quality of ALIS.
    }
    \label{fig:alis-failures}
    \vspace{-1em}
\end{figure}
