# Supplementary material for: InfinityGAN: Towards Infinite-Pixel Image Synthesis
Source: arXiv:2104.03963 source file (2022-03-11)
Supplement: Supplementary file 2 [file supp-fig_hr_samples.tex]

\begin{figure}[ht]
    \centering
    \includegraphics[width=\linewidth]{img/supp/hr-samples-tinypng/fig_000000.png}
    \vspace{-0.5em}
    \caption{
    \textbf{InfinityGAN samples training at a higher resolution.}
    We synthesize 4096$\times$4096 pixel images using InfinityGAN trained on Flickr-Landscape at 397$\times$397 pixels patches cropped from 773$\times$773 full images.
    The top and bottom rows are zoom-in view of the image.
    Note that the figure is 2$\times$ down-sampled to reduce file size.
    }
\end{figure}

\begin{figure}[ht]
    \centering
    \includegraphics[width=\linewidth]{img/supp/hr-samples-tinypng/fig_000001.png}
    \vspace{-0.5em}
    \caption{
    \textbf{InfinityGAN samples training at a higher resolution.}
    We synthesize 4096$\times$4096 pixel images using InfinityGAN trained on Flickr-Landscape at 397$\times$397 pixels patches cropped from 773$\times$773 full images.
    The top and bottom rows are zoom-in view of the image.
    Note that the figure is 4$\times$ down-sampled to reduce file size.
    }
    \label{fig:failure-twilight}
\end{figure}

\begin{figure}[ht]
    \centering
    \includegraphics[width=\linewidth]{img/supp/hr-samples-tinypng/fig_000002.png}
    \vspace{-0.5em}
    \caption{
    \textbf{InfinityGAN samples training at a higher resolution.}
    We synthesize 4096$\times$4096 pixel images using InfinityGAN trained on Flickr-Landscape at 397$\times$397 pixels patches cropped from 773$\times$773 full images.
    The top and bottom rows are zoom-in view of the image.
    Note that the figure is 4$\times$ down-sampled to reduce file size.
    }
\end{figure}

\begin{figure}[ht]
    \centering
    \includegraphics[width=\linewidth]{img/supp/hr-samples-tinypng/fig_000003.png}
    \vspace{-0.5em}
    \caption{
    \textbf{InfinityGAN samples training at a higher resolution.}
    We synthesize 4096$\times$4096 pixel images using InfinityGAN trained on Flickr-Landscape at 397$\times$397 pixels patches cropped from 773$\times$773 full images.
    The top and bottom rows are zoom-in view of the image.
    Note that the figure is 4$\times$ down-sampled to reduce file size.
    }
\end{figure}
