# Supplementary material for: InfinityGAN: Towards Infinite-Pixel Image Synthesis
Source: arXiv:2104.03963 source file (2022-03-11)
Supplement: Supplementary file 3 [file supp-fig_more_baseline.tex]

\begin{figure}[h]
    \centering
    \setlength{\tabcolsep}{1.5pt}
    
    \begin{tabular}{cccc}
        SinGAN &
        StyleGAN2 + NCI &
        StyleGAN2 + NCI + FCG &
        InfinityGAN (ours) \\
        \includegraphics[width=.24\linewidth]{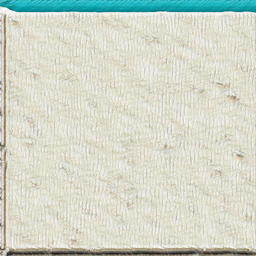} &
        \includegraphics[width=.24\linewidth]{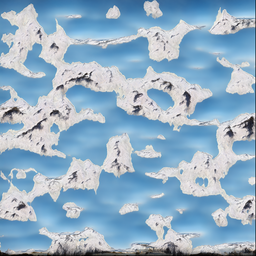} &
        \includegraphics[width=.24\linewidth]{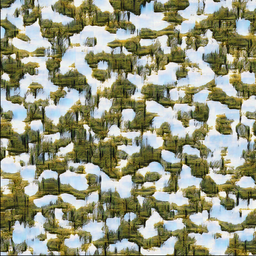} &
        \includegraphics[width=.24\linewidth]{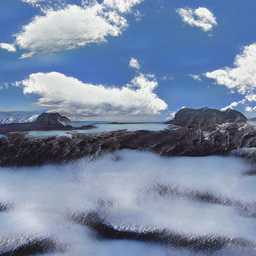} \\
        \includegraphics[width=.24\linewidth]{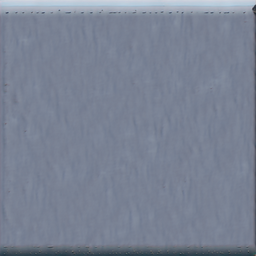} &
        \includegraphics[width=.24\linewidth]{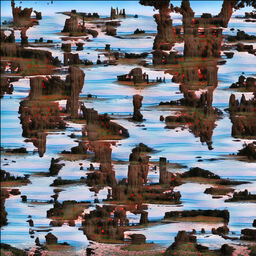} &
        \includegraphics[width=.24\linewidth]{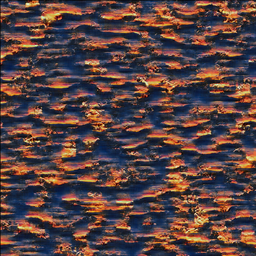} &
        \includegraphics[width=.24\linewidth]{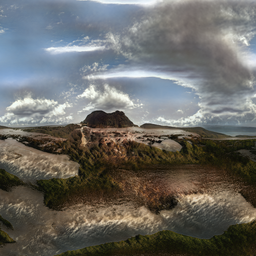} \\
        \includegraphics[width=.24\linewidth]{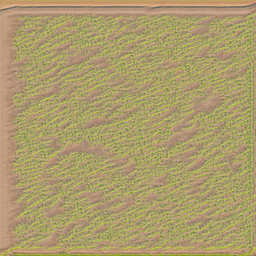} &
        \includegraphics[width=.24\linewidth]{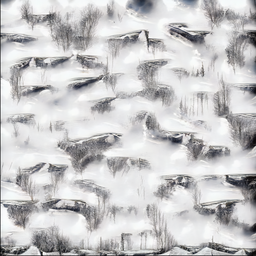} &
        \includegraphics[width=.24\linewidth]{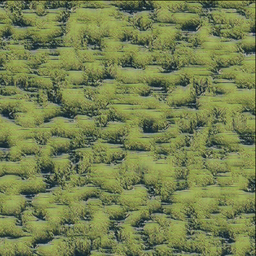} &
        \includegraphics[width=.24\linewidth]{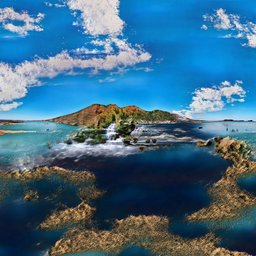} \\
        \includegraphics[width=.24\linewidth]{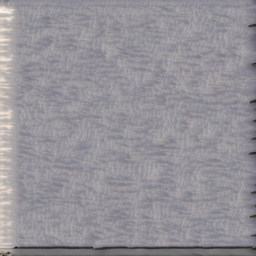} &
        \includegraphics[width=.24\linewidth]{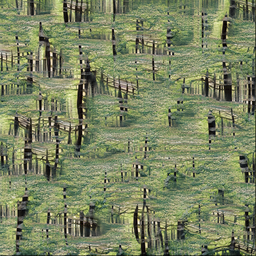} &
        \includegraphics[width=.24\linewidth]{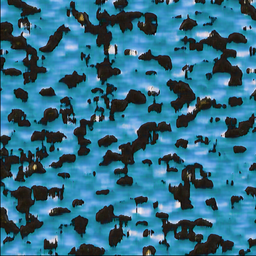} &
        \includegraphics[width=.24\linewidth]{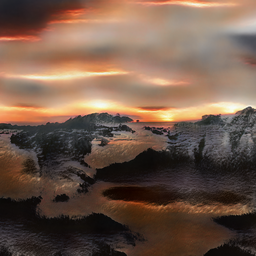} \\
        \includegraphics[width=.24\linewidth]{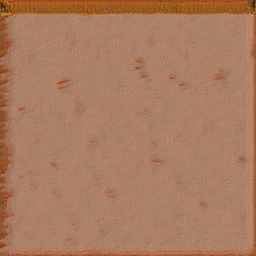} &
        \includegraphics[width=.24\linewidth]{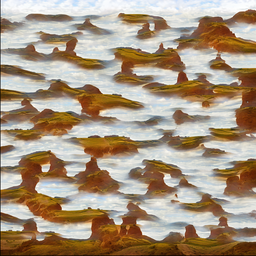} &
        \includegraphics[width=.24\linewidth]{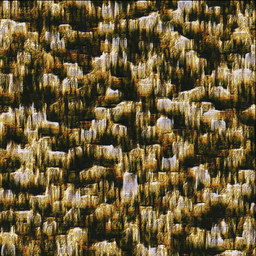} &
        \includegraphics[width=.24\linewidth]{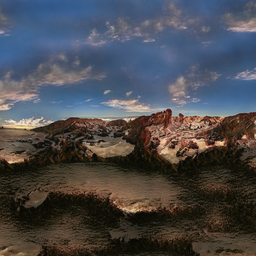} \\
    \end{tabular}
    \vspace{-0.5em}
    \caption{
    \textbf{More qualitative comparisons.}
    We show more samples on Flickr-Landscape at 1024$\times$1024 pixels.
    }
    \label{tab:my_label}
\end{figure}
