# Supplementary material for: InfinityGAN: Towards Infinite-Pixel Image Synthesis
Source: arXiv:2104.03963 source file (2022-03-11)
Supplement: Supplementary file 4 [file supp-fig_more_datasets.tex]

\begin{figure}[h]
    \vspace{10em}
    \centering
    \setlength{\tabcolsep}{1pt}
    \begin{tabular}{ccc}
        \hfill
        \multirowcell{2}[0ex][l]{
            \includegraphics[width=.08384\linewidth]{img/supp/lsun-bridge/crop.png}
        } \hfill & \hfill
        \includegraphics[width=.425\linewidth]{img/supp/lsun-bridge/000002.png} \hfill & \hfill
        \includegraphics[width=.425\linewidth]{img/supp/lsun-bridge/000006.png} \\
        &
        \includegraphics[width=.425\linewidth]{img/supp/lsun-bridge/000003.png} \hfill & \hfill
        \includegraphics[width=.425\linewidth]{img/supp/lsun-bridge/000004.png} \\
        \cmidrule(lr){1-1}
        \cmidrule(lr){2-3}
        \makecell{Training Size \\ (101$\times$101)}
        &
        \multicolumn{2}{c}{Test Size (512$\times$512)}
    \end{tabular}
    \caption{
    \textbf{LSUN bridge category.}
    InfinityGAN synthesis results at 512$\times$512 pixels on LSUN bridge category. The model is trained with 101$\times$101 pixels patches cropped from 197$\times$197 resolution real images.
    }
\end{figure}

\begin{figure}[ht]
    \vspace{2em}
    \centering
    \setlength{\tabcolsep}{1pt}
    \begin{tabular}{ccc}
        \hfill
        \multirowcell{2}[0ex][l]{
            \includegraphics[width=.08384\linewidth]{img/supp/lsun-tower/crop.png}
        } \hfill & \hfill
        \includegraphics[width=.425\linewidth]{img/supp/lsun-tower/000004.png} \hfill & \hfill
        \includegraphics[width=.425\linewidth]{img/supp/lsun-tower/000007.png} \\
        &
        \includegraphics[width=.425\linewidth]{img/supp/lsun-tower/000006.png} \hfill & \hfill
        \includegraphics[width=.425\linewidth]{img/supp/lsun-tower/000001.png} \\
        \cmidrule(lr){1-1}
        \cmidrule(lr){2-3}
        \makecell{Training Size \\ (101$\times$101)}
        &
        \multicolumn{2}{c}{Test Size (512$\times$512)}
    \end{tabular}
    \caption{
    \textbf{LSUN tower category.}
    InfinityGAN synthesis results at 512$\times$512 pixels on LSUN tower category. The model is trained with 101$\times$101 pixels patches cropped from 197$\times$197 resolution real images.
    }
\end{figure}
