# Supplementary material for: InfinityGAN: Towards Infinite-Pixel Image Synthesis
Source: arXiv:2104.03963 source file (2022-03-11)
Supplement: Supplementary file 5 [file supp-fig_more_ours1024x1024.tex]

% Unused:
% \includegraphics[width=.33\linewidth]{img/quant-plain-gen/ours1024/suppquali/000010.png} &
% \includegraphics[width=.33\linewidth]{img/quant-plain-gen/ours1024/suppquali/000014.png} &
% \includegraphics[width=.33\linewidth]{img/quant-plain-gen/ours1024/suppquali/000015.png} &
% \includegraphics[width=.45\linewidth]{img/quant-plain-gen/ours1024/suppquali/000104.png}
% \includegraphics[width=.45\linewidth]{img/quant-plain-gen/ours1024/suppquali/000023.png}
% \includegraphics[width=.45\linewidth]{img/quant-plain-gen/ours1024/suppquali/000027.png}

\begin{figure}[h]
    \vspace{2em}
    \centering
    \setlength{\tabcolsep}{1pt}
    \begin{tabular}{cc}
        
        \hfill%
        \includegraphics[width=.495\linewidth]{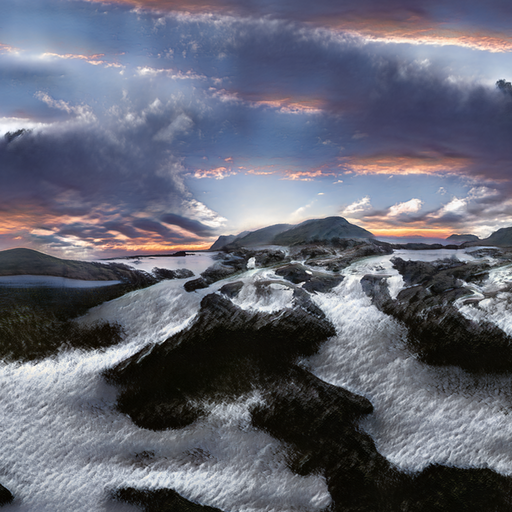} \hfill & \hfill
        \includegraphics[width=.495\linewidth]{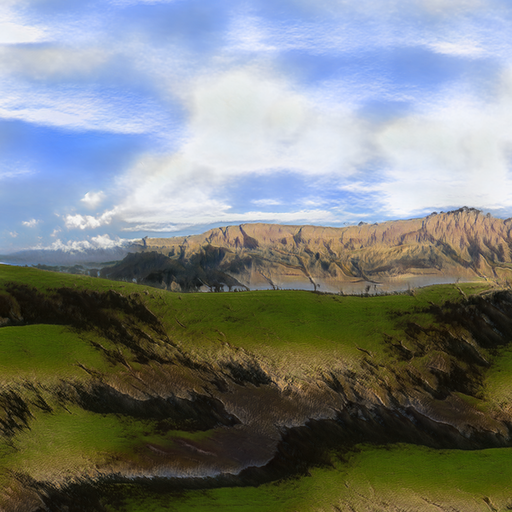} \hfill \\
        \hfill%
        \includegraphics[width=.495\linewidth]{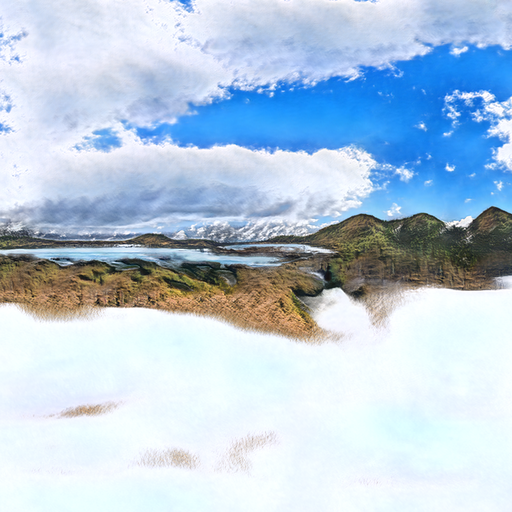} \hfill & \hfill
        \includegraphics[width=.495\linewidth]{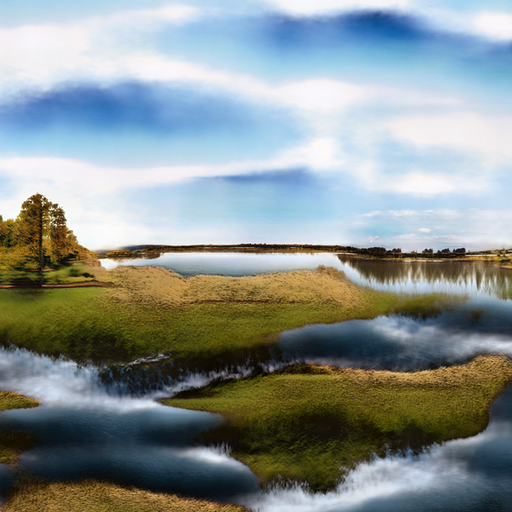} \hfill \\
    \end{tabular}
    \caption{
    \textbf{More qualitative results.}
    We provide more images synthesized at 1024$\times$1024 pixels with our InfinityGAN trained on Flickr-Landscape. All images are synthesized with the same model presented in the paper, which is trained with 101$\times$101 patches cropped from 197$\times$197 resolution real images. All images share the same coordinate and present a high structural diversity.
    Note that the images are down-sampled 2$\times$ to reduce file size.
    }
\end{figure}\clearpage

\begin{figure}[h]
    \vspace{5em}
    \centering
    \setlength{\tabcolsep}{1pt}
    \begin{tabular}{cc}
        \hfill%
        \includegraphics[width=.495\linewidth]{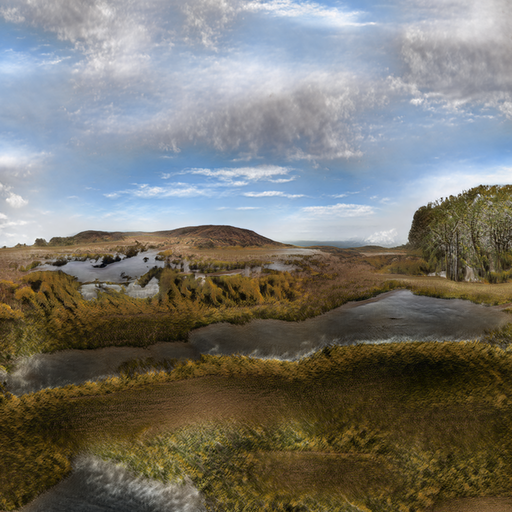} \hfill & \hfill
        \includegraphics[width=.495\linewidth]{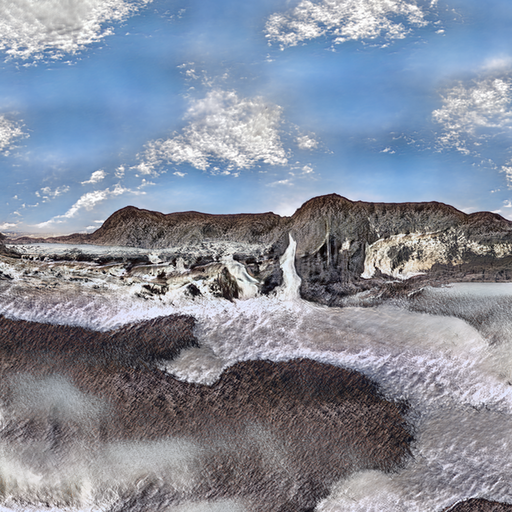} \hfill \\
        \hfill%
        \includegraphics[width=.495\linewidth]{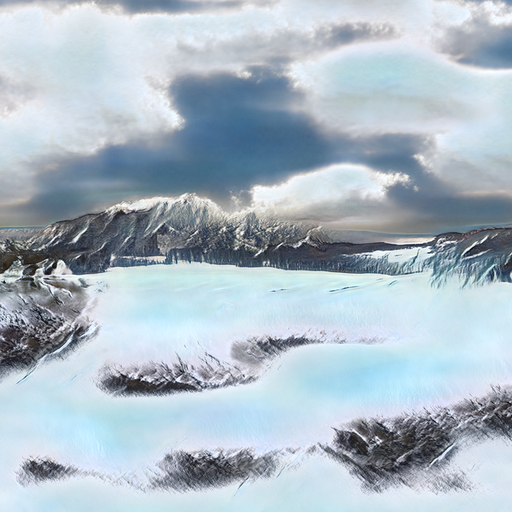} \hfill & \hfill
        \includegraphics[width=.495\linewidth]{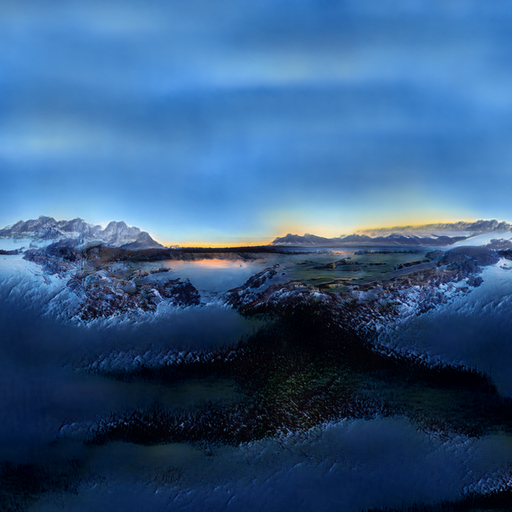} \hfill \\
    \end{tabular}
    \caption{
    \textbf{More qualitative results.}
    We provide more images synthesized at 1024$\times$1024 resolution with our InfinityGAN trained on Flickr-Landscape. All images are synthesized with the same model presented in the paper, which is trained with 101$\times$101 resolution patches cropped from 197$\times$197 resolution real images. All images share the same coordinate and present a high structural diversity.
    Note that the images are down-sampled 2$\times$ to reduce file size.
    }
    \label{fig:cloud-failure}
\end{figure}\clearpage

\begin{figure}[h]
    \vspace{5em}
    \centering
    \setlength{\tabcolsep}{1pt}
    \begin{tabular}{ccc}
        \hfill%
        \includegraphics[width=.495\linewidth]{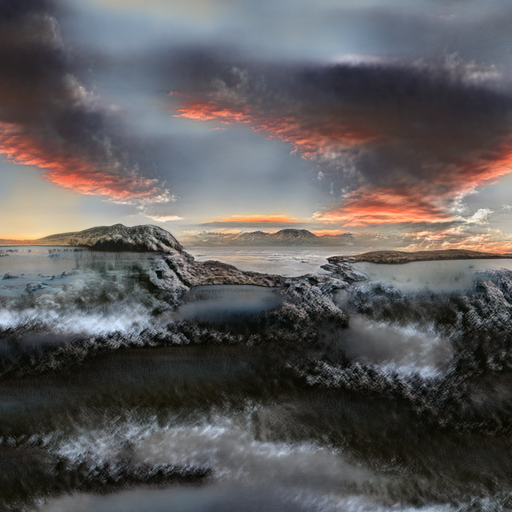} \hfill & \hfill
        \includegraphics[width=.495\linewidth]{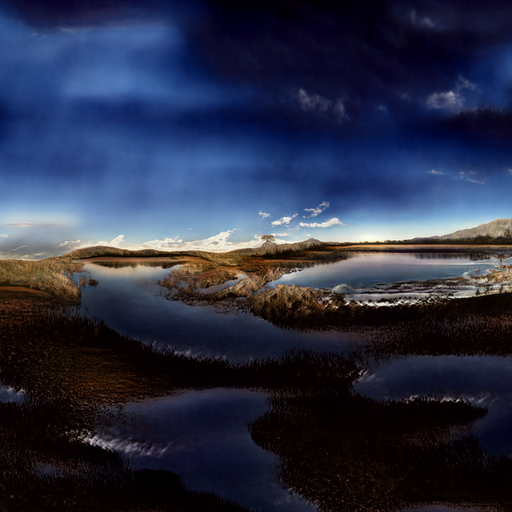} \hfill \\
        \hfill%
        \includegraphics[width=.495\linewidth]{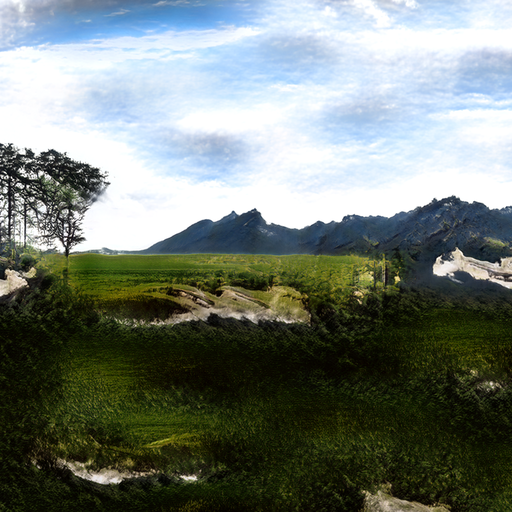} \hfill & \hfill
        \includegraphics[width=.495\linewidth]{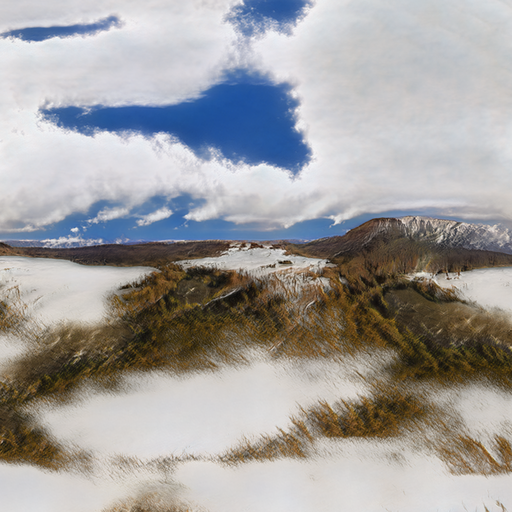} \hfill \\
    \end{tabular}
    \caption{
    \textbf{More qualitative results.}
    We provide more images synthesized at 1024$\times$1024 resolution with our InfinityGAN trained on Flickr-Landscape. All images are synthesized with the same model presented in the paper, which is trained with 101$\times$101 resolution patches cropped from 197$\times$197 resolution real images. All images share the same coordinate and present a high structural diversity.
    Note that the images are down-sampled 2$\times$ to reduce file size.
    }
    \label{fig:sunshine-failure}
\end{figure}\clearpage
