# Supplementary material for: InfinityGAN: Towards Infinite-Pixel Image Synthesis
Source: arXiv:2104.03963 source file (2022-03-11)
Supplement: Supplementary file 6 [file supp-fig_task_compare.tex]

\begin{figure}[H]
    \centering
    % \vspace{-1em}
    \includegraphics[width=\linewidth]{img/supp/task-compare-v2.pdf}
    \caption{
    (a) \textbf{Super Resolution}: The final outputs inherit the coarse structure from and share the same field-of-view with the original input condition. 
    % Image super-resolution methods~\citep{ledig2017srgan,ledig2017photo} aim at recovering high-frequency signals instead of synthesizing novel and extended structures or objects.
    %
    (b) \textbf{Texture Synthesis}: Due to coordinate encoding, objects are generated near image the border, and the center of the image is filled with repetitive textures. 
    (c) \textbf{Image Extrapolation}: Current extrapolation models tend to copy-and-paraphrase the conditional input or create mottled textural samples, leading to repetitive results especially when the outpainted region is large. 
    % Image outpainting~\citep{abdal2020image2styleganpp,liu2020infinite,sabini2018outpainting,yang2019very} is related to image inpainting~\citep{liu2018image,yu2018free} and shares similar issues that the generator tends to copy-and-paraphrase the conditional input or create mottled textural samples, leading to repetitive results especially when the outpainted region is large. 
    %
    (d) \textbf{COCO-GAN}: COCO-GAN can only synthesize samples slightly larger than its training distribution. 
    (e) \textbf{InfinityGAN}: Ours InfinityGAN can synthesize a more favorable global structure at arbitrary resolutions without an input condition.
    }
    \label{fig:task-compare}
    % \vspace{-1em}
\end{figure}
