# Supplementary material for: InfinityGAN: Towards Infinite-Pixel Image Synthesis
Source: arXiv:2104.03963 source file (2022-03-11)
Supplement: Supplementary file 8 [file supp-fig_alis_shared_context.tex]

\begin{figure}[H]
    \centering
    \includegraphics[width=\linewidth]{img/supp/alis-shared-context/7.png}
    \includegraphics[width=\linewidth]{img/supp/alis-shared-context/8.png}
    % \setlength{\tabcolsep}{0pt}
    % \begin{tabular}{c}
        
    % \end{tabular}
    
    \caption{
    \textbf{ALIS cannot synthesis with a single holistic appearance.} 
    ALIS synthesizes repetitive content if all anchors share the same latent vector.}
    \label{fig:alis-shared-context}
\end{figure}
