# Supplementary material for: InfinityGAN: Towards Infinite-Pixel Image Synthesis
Source: arXiv:2104.03963 source file (2022-03-11)
Supplement: Supplementary file 9 [file supp-fig_architecture.tex]

\begin{figure}[H]
    \centering
    \includegraphics[width=0.95\linewidth]{img/supp/detail-arch-macro.pdf}
    \vspace{-0.5em}
    \caption{
    \textbf{A high-level overview of InfinityGAN model architecture.}
    %
    % The lower-level architectures of the modules are shown in Figure~\ref{fig:supp-arch-micro}.
    }
    \label{fig:supp-arch-macro}
    
    \vspace{1em}
    
    \centering
    \includegraphics[width=0.95\linewidth]{img/supp/detail-arch-micro.pdf}
    \vspace{-0.5em}
    \caption{
    \textbf{The low-level design of each module within InfinityGAN.}
    %
    % The overview of the generator and discriminator architectures is shown in Figure~\ref{fig:supp-arch-macro}.
    }
    \label{fig:supp-arch-micro}
    \vspace{-4em}
\end{figure}
