# Supplementary material for: InfinityGAN: Towards Infinite-Pixel Image Synthesis
Source: arXiv:2104.03963 source file (2022-03-11)
Supplement: Supplementary file 10 [file supp-fig_fused_mod_demod.tex]

\definecolor{backcolor}{rgb}{0.156,0.16,0.137}
\begin{figure}[H]
\hspace{-0.060\textwidth}
\hfill
\noindent\begin{minipage}{.525\textwidth}
\input{codes/forward}
\end{minipage}
\hfill
\noindent\begin{minipage}{.525\textwidth}
\input{codes/fused_forward}
\end{minipage}
\hfill
\hspace{-0.060\textwidth}
\vspace{-1em}
\caption{
\textbf{Implementation of spatial style fusion.}
We present (left) the original StyleGAN2 forward function, and (right) a corresponding implementation for the spatial style fusion.
We align the related code blocks on the left and right.
}
\label{fig:supp_fused_mod_demod}
\end{figure}
