# Supplementary material for: InfinityGAN: Towards Infinite-Pixel Image Synthesis
Source: arXiv:2104.03963 source file (2022-03-11)
Supplement: Supplementary file 11 [file supp-fig_more_cyclic_pano.tex]

\begin{figure}[h]
    \vspace{-1em}
    \centering
    \includegraphics[width=.965\linewidth]{img/supp/cyclic_pano_composed.png}
    \vspace{-0.5em}
    \caption{
    \textbf{More cyclic panorama synthesized with model inversion.}
    By setting the same real image on two sides (marked with {\color{red}red} box) and inverting the latent variables that reconstruct the real image, InfinityGAN can naturally synthesize horizontally cyclic panoramic images with image inbetweening.
    We synthesize the 256$\times$1280 images using InfinityGAN trained on Flickr-Scenery at 101$\times$101 pixels.
    }
    \label{fig:supp-more-cyclic-pano}
    \vspace{-3em}
\end{figure}
