# Supplementary material for: InfinityGAN: Towards Infinite-Pixel Image Synthesis
Source: arXiv:2104.03963 source file (2022-03-11)
Supplement: Supplementary file 12 [file supp-fig_more_inbetween.tex]

\begin{figure}[h]
    \vspace{-1em}
    \centering
    \includegraphics[width=0.95\linewidth]{img/supp/inbetween_composed.png}
    \caption{
    \textbf{More image inbetweening with model inversion.}
    By inverting the latent variables that reconstruct the two real images on two sides (marked with {\color{red}red} box), InfinityGAN can naturally inbetween the two images arbitrarily distant away.
    We synthesize the 256$\times$1280 images using InfinityGAN trained on Flickr-Scenery at 101$\times$101 pixels.
    }
    \label{fig:supp-more-inbetween}
    \vspace{-3em}
\end{figure}
