# Supplementary material for: InfinityGAN: Towards Infinite-Pixel Image Synthesis
Source: arXiv:2104.03963 source file (2022-03-11)
Supplement: Supplementary file 13 [file supp-fig_more_outpainting.tex]

\begin{figure}[h]
    \vspace{-1em}
    \centering
    \includegraphics[width=\linewidth]{img/supp/more_outpainting_composed.png}
    \vspace{-1.5em}
    \caption{
    \textbf{More outpainting via model inversion.}
    We present more outpainting results from InfinityGAN on Flickr-Scenery.
    We invert the latent variables from 256$\times$128 pixels real images (marked with {\color{red}red} box), then outpaint 256$\times$640 area (5$\times$ real image size).
    }
    \label{fig:supp-more-outpaint}
    \vspace{-3em}
\end{figure}
