# Supplementary material for: InfinityGAN: Towards Infinite-Pixel Image Synthesis
Source: arXiv:2104.03963 source file (2022-03-11)
Supplement: Supplementary file 14 [file supp-fig_mspie_expand.tex]

\begin{figure}[H]
    \centering
    \vspace{-0.5em}
    \includegraphics[width=\linewidth]{img/supp/mspie-extend.png}
    \vspace{-0.5em}
    \caption{
    \textbf{MS-PIE creates repetitive content in the expand setting.}
    We train the no-padding StyleGAN2 with MS-PIE at 256, 384 and 512 scales, then synthesize at 1408 scale.}
    \label{fig:mspie-expand}
    \vspace{-1em}
\end{figure}
