# Supplementary material for: InfinityGAN: Towards Infinite-Pixel Image Synthesis
Source: arXiv:2104.03963 source file (2022-03-11)
Supplement: Supplementary file 15 [file supp-fig_multi_anchor.tex]

\begin{figure}[h]
    \centering
    \includegraphics[width=\linewidth]{img/supp/multi-anchor.png}
    \vspace{-0.5em}
    \caption{
    \textbf{InfinityGAN with free-form anchor placements.}
    The spatial style fusion of InfinityGAN can place any number of style centers (called anchors in ALIS) at any location. We show case (top) a five-anchor example and (bottom) the corresponding regions covered by each style center.
    }
    \label{fig:multi-anchor}
    \vspace{-0.5em}
\end{figure}
