# Supplementary material for: InfinityGAN: Towards Infinite-Pixel Image Synthesis
Source: arXiv:2104.03963 source file (2022-03-11)
Supplement: Supplementary file 16 [file supp-fig_spatial_fusion.tex]

\begin{figure}[h]
    \centering
    \includegraphics[width=\linewidth]{img/supp/reverse_calibration.pdf}
    \caption{
    \textbf{Illustration of fusion map creation procedure and spatial fusion generation.}
    With a toy architecture example  shown in (a) and a style fusion map in the pixel space (bottom of (b)), we can reversely create spatially aligned fusion maps in all intermediate layers by padding or interpolating the fusion map in the previous layer.
    Spatial style fusion in (c) uses the fusion maps to synthesize images with a natural style transition in the pixel space.
    }
    \label{fig:supp_reverse_calibration}
\end{figure}
